# Supplementary material for: PRIME: Prioritizing Interpretability in Failure Mode Extraction
Source: arXiv:2310.00164 source file (2024-03-14)
Supplement: Supplementary file 1 [file figure.tex]

\begin{figure}
  \centering
  \begin{subfigure}{1\linewidth}
    \centering
    \begin{minipage}{0.31\linewidth}
      \includegraphics[width=1\linewidth]{figures/appendix/generalization/living17_gen_n25_t50_d25.pdf}
    \end{minipage}
    \begin{minipage}{0.31\linewidth}
      \includegraphics[width=1\linewidth]{figures/appendix/generalization/living17_gen_n50_t50_d25.pdf}
    \end{minipage}
    \begin{minipage}{0.31\linewidth}
      \includegraphics[width=1\linewidth]{figures/appendix/generalization/living17_gen_n50_t50_d30.pdf}
    \end{minipage}
  \end{subfigure}\\%\vspace{10pt}
  \begin{subfigure}{1\linewidth}
    \centering
    \begin{minipage}{0.31\linewidth}
      \includegraphics[width=1\linewidth]{figures/appendix/generalization/waterbirds_gen_n25_t40_d25.pdf}
    \end{minipage}
    \begin{minipage}{0.31\linewidth}
      \includegraphics[width=1\linewidth]{figures/appendix/generalization/waterbirds_gen_n35_t40_d25.pdf}
    \end{minipage}
    \begin{minipage}{0.31\linewidth}
      \includegraphics[width=1\linewidth]{figures/appendix/generalization/waterbirds_gen_n35_t40_d30.pdf}
    \end{minipage}
  \end{subfigure}
  \begin{subfigure}{1\linewidth}
    \centering
    \begin{minipage}{0.31\linewidth}
      \includegraphics[width=1\linewidth]{figures/appendix/generalization/imagenet_gen_n30_t25_d25.pdf}
    \end{minipage}
    \begin{minipage}{0.31\linewidth}
      \includegraphics[width=1\linewidth]{figures/appendix/generalization/imagenet_gen_n30_t25_d30.pdf}
    \end{minipage}
    \begin{minipage}{0.31\linewidth}
      \includegraphics[width=1\linewidth]{figures/appendix/generalization/celeba_age_gen_n50_t200_d30.pdf}
    \end{minipage}
  \end{subfigure}\\
\caption{
    Evaluating detected failure modes on unseen (test) dataset. We extract failure modes on different datasets using different values of $(s, a)$.
}
\label{fig:gen-appendix}
\end{figure}
